# Supplementary material for: Unconditional steady-state entanglement in macroscopic hybrid systems by coherent noise cancellation
Source: arXiv:1801.02569 source file (2018-09-18)

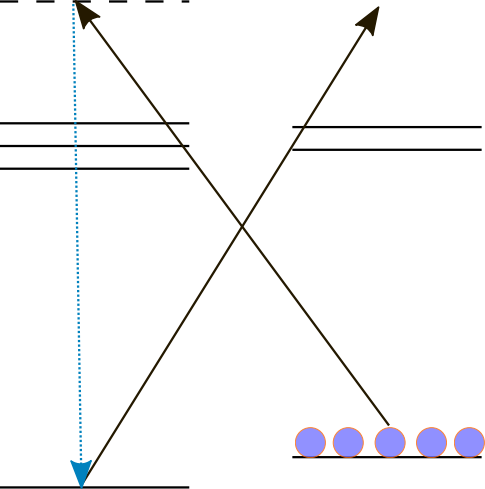

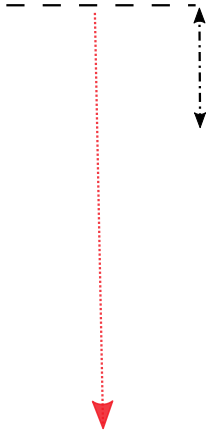

Supplement: Supplementary file 1 [file supple_fig_1_v4.pdf]
